# Supplementary material for: Proxy Methods for Domain Adaptation
Source: arXiv:2403.07442 source file (2024-03-12)
Supplement: Supplementary file 1 [file A_2_existence_m0.tex]

\subsection{Discrete Case of the Bridge Function $m_0$}

The construction of the bridge function $m_0$ in discrete setting is similar to the construction of $h_0$ introduced in~\ref{appendix:discrete_h0}. We define $P(C\mid x)=\begin{bmatrix}p(c_1\mid x)\cdots p(c_{k_C}\mid x)\end{bmatrix}^\top\in\RR^{k_C}$, $P(U\mid x)=\begin{bmatrix}p(u_1\mid x)\cdots p(u_{k_U}\mid x)\end{bmatrix}^\top\in\RR^{k_U}$ and $P(C\mid u, x)=\begin{bmatrix}p(c_1\mid u, x)\cdots p(c_{k_C}\mid u, x)\end{bmatrix}^\top\in\RR^{k_C}$ as column vectors. Let $P(C\mid U, x)=\begin{bmatrix}P(C\mid u_1,x)\cdots P(C\mid u_{k_U},x)\end{bmatrix}\in \RR^{k_C\times k_U}$ be a matrix of $p(c\mid u,x)$. The goal is to find a matrix $\tilde{M}_0(C, W, x)$ such that
\[
P(C\mid x)=\tilde{M}_0(C,W,x)P(W\mid x),\quad x\in\Xcal.
\]
Recall $W\indep X\mid U$ and hence
\begin{align}\label{eq:factor_w_x}
P(W\mid x)&=P(W\mid U, x)P(U\mid x)\notag\\
&=P(W\mid U)P(U\mid x)
\end{align}
We can write
\begin{equation}\label{eq:factor_c_x}
P(C\mid x)=P(C\mid U,x)P(U\mid x)
\end{equation}
Under Assumption~\ref{assumption:inverse}, $p(W\mid U)$ is invertible and hence combining~\eqref{eq:factor_w_x}--\eqref{eq:factor_c_x}, we arrive at
\[
P(C\mid x)=\underbrace{P(C\mid U,x)P(W\mid U)^{-1}}_{\tilde{M}_0(C,W,x)}P(W\mid x).
\]
However, contrary to $\tilde{H}_0(Y,w,c)$ which is equivalent to $\tilde{H}_0(Y,W,c)=P(Y\mid X,c)P(W\mid X,c)^{-1}$, computing $\tilde{M}_0(C,W,x)$ requires a bit more work: it requires the knowledge of $P(W\mid U)$. Once we obtain $P(W\mid U)$, we can obtain $P(C\mid U, x)$ by solving~\eqref{eq:factor_w_xc} for every $c\in\Ccal$. \citet{kuroki2014measurement} and~\citet{alabdulmohsin2023adapting} showed that $P(W\mid U)$ in Figure~\ref{fig:model} is identifiable under mild assumptions. We review the assumptions introduced in~\citet{alabdulmohsin2023adapting} and show that the bridge function $\tilde{M}_0(C,W,x)$ is identifiable without knowing $U$. 
\begin{assumption}\label{assumption:category}
The number of categories of $X,W,U$ satisfies $k_X,k_W\geq k_U$.
\end{assumption}
Assumption~\ref{assumption:category} ensures that the latent space $U$ is lower dimensional compared to observables $X,W$ and hence recovery of the latent space is possible. 
\begin{assumption}\label{assumption:distinct}
There exists a $c\in\{1,\ldots, k_C\}$ such that $p(Y\mid c, U=i)\neq p(Y\mid c, U=j)$ for $i,j\in\{1,\ldots, k_U\}$ and $i\neq j$. 
\end{assumption}
Assumption~\ref{assumption:distinct} is more technical, it ensures that the eigenvalues are distinct and hence the underlying distribution is identifiable.

\begin{proposition}\label{prop:matrix_m0} Under Assumption~\ref{assumption:CI},~\ref{assumption:inverse},~\ref{assumption:category}--\ref{assumption:distinct}, 
$\tilde{M}_0(C,W,x)$ is identifiable 
\end{proposition}

Before proving~Proposition\label{prop:matrix_m0}, we introduce the following lemma adapted from Lemma~1 in~\citet{alabdulmohsin2023adapting}.
\begin{lemma}[Adapted from Lemma~1 in~\citet{alabdulmohsin2023adapting}]\label{lemma:identifiability_discrete}
Given Assumption~\ref{assumption:CI},~\ref{assumption:category}--\ref{assumption:distinct}, all probability mass functions over $\{W,X,C,Y,\tilde{U}\}$ are identifiable, where $\tilde{U}$ is an unknown permutation of $U$. 
\end{lemma}

\begin{proof}[Proof of Proposition~\ref{prop:matrix_m0}]
    Given the result from Lemma~\ref{lemma:identifiability_discrete}, we know there exists a columnwise permutation matrix  $R$ such that
    \[
    P(W\mid U)=P(W\mid \tilde{U})R,\quad P(C\mid U,x)=P(C\mid \tilde{U},x)R.
    \]
    Therefore, we have 
    \[
    P(C\mid U,x)P(W\mid U)^{-1}=P(C\mid \tilde{U},x)P(W\mid \tilde{U})^{-1}.
    \]
    Hence we complete the identification proof. \citet{alabdulmohsin2023adapting} provided a procedure to estimate $P(W\mid \tilde{U})$ from $(W,X,Y,C)$ by solving a eigendecomposition problem. We omit the details and refer to Algorithm~1 in~\citet{alabdulmohsin2023adapting}. Once $P(W\mid \tilde{U})$ is obtained, then $P(C\mid \tilde{U}, x)$ can be obtained by solving the linear system~\ref{eq:factor_w_xc} for each $c$. 
\end{proof}

%Observe that both $P(W\mid x)$ and $P(C\mid x)$ in~\eqref{eq:factor_w_x}--\eqref{eq:factor_c_x} take the input $P(U\mid x)$ and feed into the matrices $P(W\mid U, x)$ and $P(C\mid U,x)$, respectively. We ask the question, under what conditions there exist a matrix $\tilde{M}_x$ such that we can obtain the relation 
%\begin{align*}
%    P(C\mid U, x)&=\tilde{M}_xP(W\mid U , x)=\tilde{M}_xP(W\mid U);\\
%    P(W\mid U)  &=\tilde{M}_x^*P(C\mid U , x),
%\end{align*}
%where $\tilde{M}_x^*$ is the adjoint of $\tilde{M}_x$. Assume that $\tilde{M}_x$ for $x\in\Xcal$ exists, then we can show that $\tilde{M}_x$ is a choice of $\tilde{M}_0(C,W,x)$ as
%\[
%P(C\mid x)=P(C\mid U,x)P(U\mid x)=\tilde{M}_xP(W\mid U , x)P(U\mid x)=\tilde{M}_xP(W\mid x). 
%\]
%The sufficient conditions of the existence of $\tilde{M}_x$ is answered by Picard's theorem, which holds for a more general setting of the linear systems of compact operators as we discuss in the following section.

\subsection{Existence of bridge function $m_0$}\label{appendix:existemce_m0}
First, for both $f\in\{p,q\}$, we define a new bridge function as
\[
\int_{\Wcal}{m}_0^f(w,c,x)f(w\mid c,x)dw = 1.
\]

We discuss the existence of the bridge function $m_0$ in this section. Let $f$ be either the distribution from $p$ or $q$, recall the definition
\begin{equation}\label{eq:define_m0} 
    f(c\mid x) = \int m_0(w,c,x)f(w\mid  x)dw.
\end{equation}

\begin{assumption}[Informative Proxies]\label{assumption:complete:proxy}
For any mean squared integrable function $g$, both the source domain and the target domain satisfy
$
    \EE[g(U)\mid X, W=w] = 0 
$ for all $w\in\Wcal$ if and only if $g(u)=0$ almost surely.
\end{assumption}

We will show that $m_0$ exists under Assumption~\ref{assumption:compactness}--\ref{assumption:completeness:action} and some regularity conditions by applying Picard's condition.

For all $c\in\Ccal$ and $x\in\Xcal$, define the integral operator $K_{w\mid c,x}:L_2(W\mid c,x)\rightarrow L_2(U\mid c,x)$ with the kernel function
$$
k(w,u,c,x) = \frac{f(w,u\mid c,x)}{f(w\mid c,x)f(u\mid c,x)}.
$$
Then, we can write~\eqref{eq:define_m0} as
\begin{align}\label{eq:action:bridge:ls}
f(c\mid u,x)& = \int_{\Wcal}m_0(w,c,x)f(w\mid u)dw\notag\\
&=\int_{\Wcal}m_0(w,c,x)f(w\mid u,c,x)dw& (W\indep C,X\mid U)\notag\\
 &= \int_{\Wcal} k(w,u,c,x)m_0(w,c,x)f(w\mid c,x) dw=K_{w\mid c ,x} m_0.
\end{align}
To show that the solution $m_0$ exist, we apply Picard's theorem.

\begin{assumption}\label{assumption:compactness}
$\int_{\Wcal}\int_{\Ucal} f(w\mid u,c,x)f(u\mid w,c,x)dwdu<\infty.$
\end{assumption}
This assumption is a sufficient condition for $K_{w\mid c,x}$ to be compact operator~\citep[Theorem~2.34]{carrasco2007linear}. Let $\{\lambda_j,\varphi_j,\psi_j\}_{j=1}^\infty$ be the singular system of $K_{w\mid c,x}$ and $\varphi_j\in L_2(U\mid c,x)$, $\psi_j\in L_2(W\mid c,x)$

\begin{assumption}
\label{assumption:completeness:action}
$\EE[g(c,x,U)\mid W,C=c,X=x]=0$ if and only if $g(c,x,u)=0$ almost surely.
\end{assumption}
This assumption states that $W$ capture enough information about the change of $U$. Same completeness assumption is made in constructing the control bridge function in~\citet{cui2023semiparametric}. 
%Note that Assumption~\ref{assumption:completeness:action} is weaker than Assumption~\ref{assumption:completeness} as we conditional on additional variable $W$.

\begin{proposition}[Existence of  $m_0$]\label{prop:existence_m0}
Assume that Assumption~\ref{assumption:compactness}--\ref{assumption:completeness:action} hold, and
\begin{enumerate}
    \item $f(c\mid u,x)\in L_2(U\mid c,x)$
    \item $\sum_{j}\lambda_j^2(\dotp{f(c\mid u,x)}{\varphi_j})^2<\infty$.
\end{enumerate}
Then, there exists an solution $m_0$ of~\eqref{eq:action:bridge:ls}.
\end{proposition}

\begin{proof}[Proof of Proposition~\ref{prop:existence_m0}]
    Since~\eqref{eq:action:bridge:ls} is the Fredholm integral of first kind, it suffices to verify the conditions for the Picard's theorem. Assumption~\ref{assumption:compactness} is a sufficient condition for $K_{w\mid c,x}$ to be compact operator~\citep[Theorem~2.34]{carrasco2007linear}. The next step is to verify that $\Ncal(K_{w\mid c,x}^*)^\perp=L_2(U\mid c,x)$. Note that for any $g\in L_2(U\mid c,x)$, we have
    \begin{align*}
        [K_{w\mid c,x}^*g](w,c,x)&=\int_{\Ucal} K(w,u,c,x)g(u,c,x)f(u\mid c,x)du\\
        &=\EE[g(U,c,x)\mid w,c,x].
    \end{align*}
From Assumption~\ref{assumption:completeness:action}, we see that the null space of $K_{w\mid c,x}^*$ is zero function. Hence, $\Ncal(K_{w\mid c,x}^*)^\perp=L_2(U\mid c,x)$. Then, we apply Picard's theorem, restated in Lemma~\ref{lemma:picard}, and complete the proof.
\end{proof}
