# Supplementary material for: Proxy Methods for Domain Adaptation
Source: arXiv:2403.07442 source file (2024-03-12)
Supplement: Supplementary file 2 [file B_2_transferable_m0.tex]

\subsection{Proof of Theorem~\ref{theorem:partial_iden}}
Assume that $m_0$ exists, we have for $f\in\{p,q\}$ such that
\begin{align*}
    f(c\mid x) &= \int_{\Ucal} f(c,u\mid x)du\\
    &=\int_{\Ucal} f(c\mid u,x)f(u\mid x)du\\
    &=\int_{\Ucal}\int_{\Wcal}
    m_0^f(w,c,x)f(w\mid u,x)f(u\mid x)dwdu\\
    &=\int_{\Wcal}m_0^f(w,c,x)f(w\mid x)dw&(W\indep X\mid U).
\end{align*}
Since, under Assumption~\ref{assumption:graph}, $m_0^p$ is equivalent to $m_0^q$ almost surely, we
can write
\begin{equation}\label{eq:q_m0}
q(c\mid x)=\int_{\Wcal}m_0^p(w,c,x)q(w\mid x)dw.
\end{equation}
As we can obtain $m_0^p$ by solving the Fredholm integral equation using the observable in the source domain and $(W,X)$ is observed in the target domain, we are able to identify $q(c\mid x)$. Plug the result~\eqref{eq:q_m0} into~\eqref{eq:main_identification}, we then complete the proof.   
\section{Useful Lemmas}
This section introduces useful lemmas that are used in showing the proofs in previous sections. 
\begin{lemma}[Picard's Theorem]\label{lemma:picard}
Let $K:\mathbb{H}_1\rightarrow\mathbb{H}_2$ be a compact operator with singular system $\{\lambda_j,\varphi_j,\psi_j\}_{j=1}^\infty$ and $\phi$ be a given function in $\mathbb{H}_2$. Then the equation of first kind $Kh=\phi$ have solutions if and only if
\begin{enumerate}
    \item $\phi\in\Ncal(K^*)^\perp$, where $\Ncal(K^*)=\{h:K^*h=0\}$ is the null space of the adjoint operator $K^*$.
    \item $\sum_{j=1}^{+\infty}\lambda_j^{-2}\abr{\dotp{\phi}{\psi_j}}^2<\infty$.
\end{enumerate}
\end{lemma}
