# Supplementary material for: Proxy Methods for Domain Adaptation
Source: arXiv:2403.07442 source file (2024-03-12)
Supplement: Supplementary file 3 [file C_contZ.tex]

\section{Another Framework for Multi-domain Adaptation}\label{sec:continuousz}
\begin{figure*}
    \centering
    \begin{subfigure}[t]{0.28\textwidth}
    \resizebox{!}{7 em}{\begin{tikzpicture}
    % nodes
     \node[latent, line width=.8pt] (X) {$X$};%
     \node[latent, xshift=2cm, line width=.8pt] (Y) {$Y$};%
     \node[latent, above=of C,xshift=-1cm, line width=.8pt] (Z) {$Z$};%
     \node[obs, above=of C,xshift=1cm, line width=.8pt] (U) {$U$}; %
     \node[latent,above=of Y, xshift=1cm, line width=.8pt] (W) {$W$} edge [->, line width=.8pt] (Y);%
     %\node[latent,above=of x,xshift=-1cm,fill] (y) {$y$}; %
     %\edge node {C} [dashed] node {W};
     %\draw (1,1.69) circle(.36cm);
    % plate
    % {\tikzset{plate caption/.append style={above=2pt of #1.south east}}
    %  \plate [inner sep=.1cm,xshift=-0.05cm,line width=.8pt] {plate1} {(X)(Y)(U)(W)} {$k_Z$};} %
    % edges
     \edge [line width=.8pt] {U} {X}
     \edge [line width=.8pt]{U} {W}
     \edge [line width=.8pt]{X, U} {Y}
     \edge [line width=.8pt] {Z} {U}
    %\node [fit=(X) (Y) (U) (W), inner sep=3pt, draw, line width=.5pt, rounded corners] (plate1) {};
    %\node [above left, inner sep=1pt, xshift=-4pt, yshift=2pt] at (plate1.south east) {\large $n$};
     \end{tikzpicture}}
    %\vspace{\fill}
     \caption{Multi-Domain shift}
     \label{fig:multishift}
     \end{subfigure}
\caption{Causal diagrams. $X$ is the covariate, $Y$ is the response, $C$ is the concept, $W$ is the proxy, $Z$ is the domain-related variable, and $U$ is the latent variable.  %Dashed line implies the edge can be present or absent. %Bidirected edge implies either direction is valid.
}
\label{fig:model2}
\end{figure*}
We consider a similar setting of the multi-source domain case where now the variable $Z$ is extended from a domain index to a domain-related proxy random variable. \kt{[give an example here]}
Now, we consider $P(Z)$ as the distribution of sampling across $\Zcal$.
In the source domain, we observe $(W,Z,Y,X)$ from distribution $P$. In the target domain, the distribution of $Z$ follows $Q(Z)$. In the target domain, we observe $(W,Z,X)$. Our goal is to study the problem of $\EE_q[Y\mid x]$. It is worth noting that this setting is slightly different from the multi-source setting in Section~\ref{sec:blessingsmultipledomains}, where we are studying $\EE_q[Y\mid x]=\EE_{p}[Y\mid x, z_{k+1}]$. However, the underlying analysis of this new framework bares much similarity with the analysis in the concept case in Section~\ref{ssec:identificationwconcept}. We formalize the concept by first introduce the following shift assumption.
\begin{assumption}\label{assumption:shiftz}
The shift between $P$ and $Q$ is located in $Z$, i.e., there is a shift $P(Z)\neq Q(Z)$, but $Q(U\mid Z=z)=P(U\mid Z=z)$ for all $z\in\Zcal$.
\end{assumption}

In this setting, we define the bridge function similar to~\eqref{eq:define_m0_p} and~\eqref{eq:define_m0_q}:
\begin{align}
    \EE_p[Y\mid x,z] &= \int k_0^p(w,x)\mathrm{d}P(w\mid x,z);\label{eq:k0p}\\
    \EE_q[Y\mid x,z] &= \int k_0^q(w,x)\mathrm{d}Q(w\mid x,z).\notag
\end{align}
Furthermore, marginalizing over $Z$,  we can write the optimal predictor as
\begin{align*}
    \EE_p[Y\mid x] &= \int k_0^p(w,x)\mathrm{d}P(w\mid x), \quad\EE_q[Y\mid x] = \int k_0^q(w,x)\mathrm{d}Q(w\mid x).
\end{align*}
The question is whether the bridge function $k_0^p$ can be transferred to the target domain. To do this, we make the following completeness assumption. 
\begin{assumption}
[Informative variables] \label{assumption:completenes2} Let $g$ be any mean squared integrable function. Both the source domain and the target domain, $(f,F)\in\{(p,P), (q,Q)\}$, satisfy 
$
    \EE_f[g(U)\mid z,x] = 0 
$ for all $x\in\Xcal, z\in\Zcal$ if and only if $g(U)=0$ almost surely with respect to $F(U)$.
\end{assumption}
With this completeness assumption and additional structured assumption, we can show the following proposition. 
\begin{proposition}\label{prop:identifymultisouce2} Assume that $k_0^p, k_0^q$ exist and under Assumption~\ref{assumption:graph}, \ref{assumption:CI}, \ref{assumption:support_target}, \ref{assumption:shiftz}, \ref{assumption:completenes2}, we can write
\[
    \EE_q[Y\mid x] = \int k_0^p(w,x)\mathrm{d}Q(w\mid x),
\]
for all $x\in \Xcal$. 
\end{proposition}
Along with~\eqref{eq:k0p}, the proposition tells that if we observe $(W,X,Y,Z)$, we can identify $k_0^p$ and observing $(W,X)$ in the target domain allows us to compute the quantity of $\EE_q[Y\mid x]$ for all $x\in\Xcal$. Perhaps this result does not come as a surprise because the setting is the same as the setting of the concept case discussed in Figure~\ref{fig:shiftwconcepts} except now we are identifying the quantity $\EE_q[Y\mid c]$ in  Figure~\ref{fig:shiftwconcepts} as compared to $\EE_q[Y\mid x]$ in Section~\ref{ssec:identificationwconcept}. The major difference is that in the current setting, we only require observing $(W,X)$ in the target domain for domain adaptation whereas the concept case in Section~\ref{ssec:identificationwconcept} requires observing $(W,X,C)$ in the target domain.

{\bf Comparison of the two multi-domain adaptation frameworks.} We discuss two different frameworks for the multi-domain adaptation stemmed from the proxy method~\citep{miao2018identifying}. In the setting of Proposition~\ref{prop:identifymultisouce2}, we require domain-related proxies $Z$  and the shift happens in $Z$ as stated in Assumption~\ref{assumption:shiftz}. In contrast, the multi-domain setting discussed in Section~\ref{sec:blessingsmultipledomains} uses the domain index as $Z$ and makes assumption that $P(U\mid z)\neq P(U\mid z')$ for $z'\neq z$.  In the case when we do not have domain-related proxy random variables, we might use the method developed in Section~\ref{sec:blessingsmultipledomains}. However, the completeness condition, namely  Assumption~\ref{assumption:completeness_z},  may fail to be satisfied when $U$ have high-dimensions,  and $P(U\mid x,z)$ is complex (see~Appendix of ~\citet{miao2022identifying} and references therein for discussion of the sufficient conditions of completeness condition). Under this setting, we need more `informative' $Z$ that provides the variability of $U$ than domain index. Hence, we might need domain-related proxies that are potentially high-dimensional and continuous. Hence, the new framework studied in Proposition~\ref{prop:identifymultisouce2} is more preferable.

\begin{proof}[Proof of Proposition~\ref{prop:identifymultisouce2}]
Under Assumption~\ref{assumption:graph},~\ref{assumption:completenes2}, following the same argument as the proof of Theorem~\ref{theorem:complete_identification} in Appendix~\ref{ssec:theorem:concept}, we argue that for every $x\in\Xcal, u\in\Ucal$ such that $Q(u), P(u)>0$ we have
\[
\int k_0^p(w,x)\mathrm{d}P(w\mid u) = 
\int k_0^q(w,x)\mathrm{d}P(w\mid u).
\]
Define the support of $U$
Now, under Assumption~\ref{assumption:support_target}, we could use the same trick as shown in the proof of Theorem~\ref{ssec:theorem:concept} in Appendix~\ref{theorem:complete_identification} and obtain
\begin{align*}
\EE_q[Y\mid x] &= \int_{\Zcal}\int_{\Ucal}\cbr{\int_{\Wcal} k_0^q(w,x)\mathrm{d}P(w\mid u)}\mathrm{d}Q({u\mid z,x})\mathrm{d}Q(z\mid x)\\
&= \int_{\Zcal}\int_{\Ucal}\cbr{\int_{\Wcal} k_0^p(w,x)\mathrm{d}P(w\mid u)}\mathrm{d}Q({u\mid z,x})\mathrm{d}Q(z\mid x).
\intertext{Apply Fubini's theorem, we can write the above display as}
&={\int_{\Wcal}\int_{\Ucal} k_0^p(w,x)\mathrm{d}P(w\mid u)}\int_{\Zcal}\mathrm{d}Q({u\mid z,x})\mathrm{d}Q(z\mid x)\\
&=\int_{\Wcal}k_0^p(w,x)\mathrm{d}Q(w\mid x) = \EE_q[k_0^p(W,x)\mid x]. 
\end{align*}

\end{proof}

%However, it comes as no surprise that the underlying analysis is similar as we frame $Z$ in Section~\ref{sec:blessingsmultipledomains} as an exogenous variable
