# Supplementary material for: Proxy Methods for Domain Adaptation
Source: arXiv:2403.07442 source file (2024-03-12)
Supplement: Supplementary file 4 [file E_2_deepkernel_partial.tex]

\subsection{Deep Partial Adaptation}
For partial adaptation, in addition to learn $h_0$, we need to learn the second bridge function $m_0$. We will discuss the procedure to learn $m_0$ in the following.

\textbf{Training on source domain.} Recall form~\eqref{eq:defineA} that $\EE[\phi(C)\mid x]=A[\EE[\phi(W)\mid x]\otimes\phi(x)]$. Replace the feature functions with neural nets, we consider the following bridge function and conditional mean embed:
\begin{align*}
    \EE[\Psi_{\theta_{W_2}}(W)\mid x]&=F\Psi_{\theta_{X_4}}(x);\\
    \EE[\Psi_{\theta_{C_3}}(C)\mid x]&=A(\EE[\Psi_{\theta_{W_2}}(W)\mid x]\otimes\Psi_{\theta_{X_5}}(x)),
\end{align*}
where $F\in\RR^{d_w\times d_x}$, $A\in\RR^{d_c\times (d_wd_x)}$, and $\Psi_{\theta_{X_4}}, \Psi_{\theta_{X_5}}(x)$ are neural nets. Noting that $\Psi_{\theta_{W_2}}$ and $\Psi_{\theta_{C_3}}(C)$ are the feature nets trained in \emph{Step 2} of the full graph adaptation procedure. To learn the parameters, we add additional two steps to the training procedure with training samples $\{(x_i^4,w_i^4)\}_{i=1}^{m_4}$ and $\{(x_i^5, c_i^5,w_i^5)\}_{i=1}^{m_5}$.

\emph{Step 4}. In this step, we want estimate $\EE[\Psi_{\theta_{W_2}}(W)\mid x]=F\Psi_{\theta_{X_4}}(x)$. Given $\lambda_4>0$, the objective function is
\[
\Lcal_4(F, \theta_{X_4})=\frac{1}{m_4}\sum_{i=1}^{m_4}\|\Psi_{\theta_{W_2}}(w_i^4)-F\Psi_{\theta_{X_4}}(x_i^4)\|_2^2+\lambda_4\|F\|_F^2.
\]
Repeat similar procedure as \emph{Step 1}, we will obtain $(\hat{F}, \hat{\Psi}_{\theta_{X_4}})$. 

\emph{Step 5}. Finally, to estimate $\EE[\Psi_{\theta_{C_3}}(C)\mid x]$, we optimize
\[
\Lcal_5(A, \theta_{X_5})=\frac{1}{m_5}\sum_{i=1}^{m_5}\|\Psi_{\theta_{C_3}}(c_i^5)-A(F\Psi_{\theta_{X_4}}(x_i^5)\otimes\Psi_{\theta_{X_5}}(x_i^5))\|_2^2+\lambda_5\|A\|_F^2.
\]
Repeat similar procedure as \emph{Step 1}, we will obtain $(\hat{A}, \hat{\Psi}_{\theta_{X_5}})$.

\textbf{Training on target domain.} To adapt to the shifts, it requires to learn the conditional mean embedding in the target domain: 
\[
    \EE_q[\Psi_{\theta_{W_2}}(W)\mid x]=F_q\Psi_{\theta_{X_4}^q}(x).
\]
Repeat \emph{Step 4} with samples from the target domain, we will obtain $(\hat{F}_q, \hat{\Psi}_{\theta_{X_4}}^q)$.  Then, given a new sample $x_{\text{new}}$ from the target domain, the partial prediction is
\[
\hat{y}=\hat{D}(\hat{A}(\hat{F}_q\hat{\Psi}_{\theta_{X_4}^q}(x_{\text{new}})\otimes\hat{\Psi}_{\theta_{X_5}}(x_{\text{new}}))\otimes\hat{F}_q\hat{\Psi}_{\theta_{X_4}^q}(x_{\text{new}})).
\]
