# Supplementary material for: Proxy Methods for Domain Adaptation
Source: arXiv:2403.07442 source file (2024-03-12)
Supplement: Supplementary file 5 [file E_deepkernel.tex]

\section{Deep Feature Adaptation}
In this section, we introduce the adaptation method where the kernel function is replaced by deep neural networks. The methodology is motivated by prior results on training deep features of instrumental variable regression~\citep{xu2020learning} and proximal causal learning~\citep{xu2021deep}. The deep feature as opposed to predefined kernel function, is more flexible and allows practitioners to work on high-dimensional data such as images.

\subsection{Deep Full Adaptation}

We first discuss the implementation of the full adaptation case as discussed in Theorem~\ref{theorem:complete_identification}.  
Let $p_x,p_w,p_c,p_y$ be the dimension of $W, X, C$ and $Y$, respectively. Let $d_x,d_w,d_c$ be the feature dimension of $W,X$ and $C$, respectively. 

\textbf{Training on source domain.} We consider the following models of the bridge function and the conditional feature means embedded by neural nets:
\begin{align*}
h_0(c,w)&=D(\Psi_{{\theta_{C_3}}}(c)\otimes \Psi_{{\theta_{W_2}}}(w));\\
\EE[\Psi_{{\theta_{W_2}}}(W)\mid x,c]&=V(\Psi_{{\theta_{C_2}}}(c)\otimes\Psi_{{\theta_{X_2}}}(x));\\
\EE[\Psi_{{\theta_{C_3}}}(C)\otimes\Psi_{{\theta_{W_2}}}(W)\mid x]&=Z\Psi_{{\theta_{X_1}}}(x),
\end{align*}
where $D\in\RR^{p_y\times(d_cd_w)}$, $V\in\RR^{d_w\times(d_cd_x)}$, $Z\in\RR^{d_cd_w\times d_x}$. Additionally, $\Psi_{{\theta_{W_2}}}, \Psi_{{\theta_{C_2}}}, \Psi_{{\theta_{C_3}}}, \Psi_{{\theta_{X_2}}}$, $\Psi_{{\theta_{X_1}}}$ are neural nets.  Therefore, we can write
\begin{align*}
\EE[h_0(c,W)\mid x, c]&=D\EE[\Psi_{{\theta_{C_3}}}(c)\otimes \Psi_{{\theta_{W_2}}}(W)\mid x, c]\\
&=D\EE[\Psi_{{\theta_{C_3}}}(c)\otimes V(\Psi_{{\theta_{C_2}}}(c)\otimes\Psi_{{\theta_{X_2}}}(x))\mid x,c].
\end{align*}

Finally, taking the expectation conditioned on $x$, we arrive at
\begin{align*}
\EE[h_0(C,W)\mid x]&=D\EE\sbr{\EE[\Psi_{{\theta_{C_3}}}(c)\otimes V(\Psi_{{\theta_{C_2}}}(c)\otimes\Psi_{{\theta_{X_2}}}(x))\mid x,c]\mid x}\\
&=DZ\Psi_{{\theta_{X_1}}}(x).
\end{align*}

Hence, to learn the parameters $D, V, Z, \Psi_{{\theta_{W_2}}}, \Psi_{{\theta_{C_2}}}, \Psi_{{\theta_{C_3}}}, \Psi_{{\theta_{X_2}}}, \Psi_{{\theta_{X_1}}}$, we construct a $3$-step alternating minimization following similar estimation procedures developed in~\citet{xu2020learning, xu2021deep}. We split the traning samples into $3$ batches: $\{(x_i^1, w_i^1,c_i^1)\}_{i=1}^{m_1}, \{(x_i^2, y_i^2,c_i^2)\}_{i=1}^{m_2}$, and $\{(x_i^3, w_i^3,c_i^3)\}_{i=1}^{m_3}$.

\emph{Step 1}. In the first step, we want to estimate the conditional mean embedding $\EE[\Psi_{{\theta_{W_2}}}(W)\mid x,c]=V(\Psi_{{\theta_{C_2}}}(c)\otimes\Psi_{{\theta_{X_2}}}(x))$ by freezing the neural net $\Psi_{\theta_{W_2}}$ and optimize the parameters $V, \theta_{C_2}, \theta_{X_2}$:
\[
\Lcal_1(V, \theta_{C_2}, \theta_{X_2})=\frac{1}{m_1}\sum_{i=1}^{m_1}\left\|\Psi_{{\theta_{W_2}}}(w_i^1)-V(\Psi_{\theta_{C_2}}(c_i^1)\otimes \Psi_{\theta_{X_2}}(x_i^1))\right\|_2^2+\lambda_1\|V\|_F^2,
\]
where $\lambda_1>0$ is the regularization parameter. 
To optimize $\Lcal_1(V, \theta_{C_2}, \theta_{X_2})$ we perform alternating minimization between $V$ and $\theta_{C_2}, \theta_{X_2}$. Consider the $t$-th iteration, we can obtain $V$ by solving the least squares:
\[
{V}^{(t+1)}=\argmin_{V}\frac{1}{m_1}\sum_{i=1}^{m_1}\left\|\Psi_{{\theta_{W_2}}}(w_i^1)-V(\Psi_{\theta_{C_2}}^{(t)}(c_i^1)\otimes \Psi_{\theta_{X_2}}^{(t)}(x_i^1))\right\|_2^2+\lambda_1\|V\|_F^2.
\]
Then take the gradient of
\[
\frac{1}{m}\sum_{i=1}^m\left\|\Psi_{{\theta_{W_2}}}(w_i^1)-{V}^{(t+1)}(\Psi_{\theta_{C_2}}^{(t)}(c_i^1)\otimes \Psi_{\theta_{X_2}}^{(t)}(x_i^1))\right\|_2^2+\lambda_1\|V\|_F^2,
\]
and back propagate on $\Psi_{\theta_{C_2}}$ and $\Psi_{\theta_{X_2}}$, we complete one step optimization. We iterate for $T_1$ steps and output $(\hat{\Psi}_{\theta_{C_2}}, \hat{\Psi}_{\theta_{X_2}})$. 

\emph{Step 2}. In the second step, we want to estimate $h_0(w,c)=D(\Psi_{{\theta_{C_3}}}(c)\otimes \Psi_{{\theta_{W_2}}}(w))$. Recall that 
$$\EE[h_0(c,W)\mid x, c]=D\EE[\Psi_{{\theta_{C_3}}}(c)\otimes V(\Psi_{{\theta_{C_2}}}(c)\otimes\Psi_{{\theta_{X_2}}}(x))\mid x,c],$$
and hence we freeze the neural net $\Psi_{{\theta_{C_2}}}$ and $\Psi_{{\theta_{X_2}}}$ and optimize
\[
\Lcal_2(D, \theta_{C_3},\theta_{{W}_2})=\frac{1}{m_2}\sum_{i=1}^{m_2}\cbr{y_i^2-D\rbr{\Psi_{\theta_{C_2}}(c_i^2)\otimes \tilde{V}(\Psi_{\theta_{C_2}}(c_i^2)\otimes \Psi_{\theta_{X_2}}(x_i^2))}}^2+\lambda_2\|D\|_F^2,
\]
where $
\tilde{V}=\argmin_{V}\frac{1}{m_1}\sum_{i=1}^{m_1}\left\|\Psi_{{\theta_{W_2}}}(w_i^1)-V(\Psi_{\theta_{C_2}}(c_i^1)\otimes \Psi_{\theta_{X_2}}(x_i^1))\right\|_2^2+\lambda_1\|V\|_F^2.
$ is a function of $\Psi_{\theta_{W_2}}$. To optimize $\Lcal_2(D, \theta_{C_3},\theta_{{W}_2})$, we take the same alternating procedure as in~\emph{Step~1}. At the $t$-th iteration, we take
\[
D^{(t+1)}=\argmin_{D}\Lcal_2(D, \theta_{C_3}^{(t)},\theta_{{W}_2}^{(t)}),
\]
and take the gradient of $\Lcal_2(D^{(t+1)}, \theta_{C_3}^{(t)},\theta_{{W}_2}^{(t)})$ and back propagate to $\Psi_{\theta_{C_3}}$ and $\Psi_{\theta_{W_2}}$. After $T_2$ iterations, we output $(\hat{\Psi}_{\theta_{C_3}}, \hat{\Psi}_{\theta_{W_2}})$. 

\emph{Step 3.}  In this step, we want to estimate $\EE[\Psi_{{\theta_{C_3}}}(C)\otimes\Psi_{{\theta_{W_2}}}(W)\mid x]=Z\Psi_{{\theta_{X_1}}}(x)$ and the objective function is
\[
\Lcal_3(Z, {\theta_{X_1}})=\frac{1}{m_3}\sum_{i=1}^{m_3}\|\Psi_{{\theta_{C_3}}}(c_i^3)\otimes\Psi_{{\theta_{W_2}}}(w_i^3)-Z\Psi_{\theta_{X_1}}(x_i^3)\|_2^2+\lambda_3\|Z\|_F^2.
\]
Again, we use alternating minimization to optimize $\Lcal_3(Z, \Psi_{\theta_{X_1}})$, same as \emph{Step 1}. 
We iterate between $\emph{Step 1--3}$ until convergence and output $(\hat{D}, \hat{V}, \hat{Z}, \hat{\Psi}_{{\theta_{W_2}}}, \hat{\Psi}_{{\theta_{C_2}}}, \hat{\Psi}_{{\theta_{C_3}}}, \hat{\Psi}_{{\theta_{X_2}}}, \hat{\Psi}_{{\theta_{X_1}}})$.

\textbf{Training on target domain.} To adapt to the target distribution, we need to estimate the conditional mean embedding 
\[
\EE_q[\Psi_{{\theta_{C_3}}}(C)\otimes\Psi_{{\theta_{W_2}}}(W)\mid x]=Z_q\Psi_{{\theta_{X_1}^q}}(x),
\]
where we want to estimate $Z_q$ and $\Psi_{{\theta_{X_1}^q}}$. The feature nets $\Psi_{{\theta_{C_3}}}$ and $\Psi_{{\theta_{W_2}}}$ are trained in the source domain and freezed when training in the target domain. This step is the same as \emph{Step 3} but with training samples replaced by from the target domain. Then, given a new sample $x_{\text{new}}$ from the target domain, the prediction is
\[
\hat{y}=\hat{D}\hat{Z}_q\hat{\Psi}_{{\theta_{X_1}^q}}(x_{\text{new}}).
\]

\subsection{Deep Multi-Source}
